# Supplementary material for: Environment-Driven Emergence of Higher-Order Collective Behavior
Source: arXiv:2602.15256 source file (2026-12-01)
Supplement: Supplementary file 1 [file 2026_nature_supplementalmaterial_preprint.pdf]

# Supplemental Material for "Environment-Driven Emergence of Higher-Order Collective Behavior"


Felipe S. Abril-Bermúdez,[1,*] David N. Fisher,[2,†] Jean-Baptiste Gramain,[1,‡] and Francisco J. Pérez-Reche[1,§]

[1] *School of Natural and Computing Sciences, University of Aberdeen, Aberdeen AB24 3UE, United Kingdom.*

[2] *School of Biological Sciences, University of Aberdeen, Aberdeen, AB243FX, United Kingdom*


### Appendix A: O-information of three Gaussian random variables

The O-information ($\Omega(\boldsymbol{z})$) for a set of $N$ random variables $\boldsymbol{z} = (z_1, z_2, \ldots, z_N)$ is defined through the difference between the total correlation $\mathrm{TC}(\boldsymbol{z})$ and the dual total correlation $\mathrm{DTC}(\boldsymbol{z})$ as [1]

$$\Omega(\boldsymbol{z}) := \mathrm{TC}(\boldsymbol{z}) - \mathrm{DTC}(\boldsymbol{z}) = (N-2)\,\mathrm{H}(\boldsymbol{z}) + \sum_{k=1}^{N} \left[\mathrm{H}(z_k) - \mathrm{H}(\boldsymbol{z}_{-k})\right]. \tag{A1}$$

Thence, it is said a system is redundancy-dominated if $\Omega > 0$, meaning lower-order constraints best capture its interdependencies. Conversely, the system is synergy-dominated if $\Omega < 0$, indicating that informational structures emerge only in the joint configuration, not in lower-order marginals. This makes $\Omega$ a useful metric for identifying emergent collective behavior for $N \geq 3$ since in general $\Omega(z_1, z_2) = \Omega(z_1) = 0$, i.e., the O-information is a practical measure for characterizing the higher-order interactions.

Now, consider three random variables $z_1$, $z_2$, $z_3$. The vector $\boldsymbol{z} = (z_1, z_2, z_3)^T$ follows a multivariate normal distribution with mean $\boldsymbol{M}$ and covariance matrix $\boldsymbol{C}$ if its joint probability density function is

$$G(\boldsymbol{z}) = \frac{1}{\sqrt{(2\pi)^3 \det(\boldsymbol{C})}} e^{-\frac{1}{2}(\boldsymbol{z}-\boldsymbol{M})^T \boldsymbol{C}^{-1} (\boldsymbol{z}-\boldsymbol{M})}. \tag{A2}$$

In this case, we write $\boldsymbol{z} \sim \mathcal{N}(\boldsymbol{M}, \boldsymbol{C})$.

To estimate the O-information of a multivariate normal distribution, recall that its marginals are also multivariate normal, obtained by discarding those that are not marginalized from the mean vector and covariance matrix [2]. This gives the following hierarchy of marginal distributions:

- $z_1 \sim \mathcal{N}(M_1, C_{11})$.
- $z_2 \sim \mathcal{N}(M_2, C_{22})$.
- $z_3 \sim \mathcal{N}(M_3, C_{33})$.
- $(z_1, z_2) \sim \mathcal{N}\left(\begin{pmatrix} M_1 \\ M_2 \end{pmatrix}, \begin{pmatrix} C_{11} & C_{12} \\ C_{12} & C_{22} \end{pmatrix}\right)$.
- $(z_1, z_3) \sim \mathcal{N}\left(\begin{pmatrix} M_1 \\ M_3 \end{pmatrix}, \begin{pmatrix} C_{11} & C_{13} \\ C_{13} & C_{33} \end{pmatrix}\right)$.
- $(z_2, z_3) \sim \mathcal{N}\left(\begin{pmatrix} M_2 \\ M_3 \end{pmatrix}, \begin{pmatrix} C_{22} & C_{23} \\ C_{23} & C_{33} \end{pmatrix}\right)$.

Additionally, from the property $\mathbb{E}\left[(\boldsymbol{z}-\boldsymbol{M})(\boldsymbol{z}-\boldsymbol{M})^T \boldsymbol{C}^{-1}\right] = \mathbb{E}\left[\boldsymbol{C}\boldsymbol{C}^{-1}\right] = N$, where $N$ is the dimensionality of the distribution, the Shannon entropy (measured in bits) is given [3]

$$\mathrm{H}(\boldsymbol{z}) = \frac{N}{2}\log_2(4\pi) + \frac{1}{2}\log_2(\det(\boldsymbol{C})). \tag{A3}$$


[*] felipe.abrilbermudez@abdn.ac.uk
[†] david.fisher@abdn.ac.uk
[‡] jbgramain@abdn.ac.uk
[§] fperez-reche@abdn.ac.uk

Therefore, the O-information estimated from Eq. (A1) is

$$\begin{aligned}\Omega(z_1,z_2,z_3) &= \mathrm{H}\left(z_1,z_2,z_3\right)+\mathrm{H}\left(z_1\right)-\mathrm{H}\left(z_2,z_3\right)+\mathrm{H}\left(z_2\right)-\mathrm{H}\left(z_1,z_3\right)+\mathrm{H}\left(z_3\right)-\mathrm{H}\left(z_1,z_2\right)\\ &= \mathrm{H}\left(z_1,z_2,z_3\right)+\mathrm{H}\left(z_1\right)+\mathrm{H}\left(z_2\right)+\mathrm{H}\left(z_3\right)-\mathrm{H}\left(z_1,z_2\right)-\mathrm{H}\left(z_1,z_3\right)-\mathrm{H}\left(z_2,z_3\right)\\ &= \frac{1}{2}\log_2\left(\frac{\det(\boldsymbol{C})\;C_{11}\;C_{22}\;C_{33}}{(C_{11}C_{22}-C_{12}^2)(C_{11}C_{33}-C_{13}^2)(C_{22}C_{33}-C_{23}^2)}\right).\end{aligned} \tag{A4}$$

It is convenient to express the O-information as a function of three correlation coefficients

$$\rho_{12}=\frac{C_{12}}{\sqrt{C_{11}C_{22}}},\ \rho_{13}=\frac{C_{13}}{\sqrt{C_{11}C_{33}}},\ \rho_{23}=\frac{C_{23}}{\sqrt{C_{22}C_{33}}}, \tag{A5}$$

as follows

$$\Omega(z_1,z_2,z_3)=\frac{1}{2}\log_2\left(\frac{1+2\rho_{12}\rho_{13}\rho_{23}-\rho_{12}^2-\rho_{13}^2-\rho_{23}^2}{(1-\rho_{12}^2)\,(1-\rho_{13}^2)\,(1-\rho_{23}^2)}\right). \tag{A6}$$

Basic algebraic manipulations show that the sign of the O-information is identical to the sign of the functional

$$g\left[\rho_{12},\rho_{13},\rho_{23}\right]=2\rho_{12}\rho_{13}\rho_{23}-\rho_{12}^2\rho_{13}^2-\rho_{12}^2\rho_{23}^2-\rho_{13}^2\rho_{23}^2+\rho_{12}^2\rho_{13}^2\rho_{23}^2, \tag{A7}$$

subject to the constraint $g^* = 1+2\rho_{12}\rho_{13}\rho_{23}-\rho_{12}^2-\rho_{13}^2-\rho_{23}^2 > 0$ which is simpler to analyze than Eq. (A6). Indeed, $g^* > 0$ is precisely the condition ensuring positive definiteness of the covariance matrix $\boldsymbol{C}$, since in terms of the correlation matrix, we have

$$0<\det\left(\boldsymbol{C}\right)=C_{11}^2C_{22}^2C_{33}^2\ \det\begin{pmatrix}1 & \rho_{12} & \rho_{13}\\ \rho_{12} & 1 & \rho_{23}\\ \rho_{13} & \rho_{23} & 1\end{pmatrix}=C_{11}^2C_{22}^2C_{33}^2\ g^*\ \Leftrightarrow\ g^*>0\ , \tag{A8}$$

and the minors of the matrix are also non-negative, thus satisfying Sylvester's criterion for positive definiteness of $\boldsymbol{C}$.

Note that $g\left[\rho_{12},\rho_{13},\rho_{23}\right]$ preserves the symmetries of the O-information in terms of the correlation coefficients. More explicitly, the functional is invariant under elements of $S_3\times V_4$. Here, $S_3$ is the symmetric group of degree 3 associated with the invariance under any permutation of indices $(\{12\},\{13\},\{23\})$ and $V_4=\{(\epsilon_1,\epsilon_2,\epsilon_3)|\epsilon_i=\pm1,\epsilon_1\epsilon_2\epsilon_3=1\}$ is the Klein four-group associated with the invariance under even parity.

These expressions underlie the geometric partition of correlation space discussed in the main text and shown in Fig. 2 of the main text.

### Appendix B: Analytical solution in the absence of deterministic interactions ($m(\boldsymbol{z})=0$)

Consider the matrix form of the stochastic differential equations describing the dynamical model for the variables $\boldsymbol{z}=(z_1,z_2,z_3)^T$ defined in the main text:

$$d\boldsymbol{z}(t)=\boldsymbol{M}(\boldsymbol{z})\ dt+\boldsymbol{F}(t)\ d\boldsymbol{W}(t) \tag{B1}$$

where $\boldsymbol{W}(t)=(W,W_1,W_2,W_3)^T$, and

$$\boldsymbol{M}(\boldsymbol{z})=\begin{pmatrix}\mu_1+m(\boldsymbol{z})\\ \mu_2\\ \mu_3\end{pmatrix},\qquad \boldsymbol{F}(t)=\begin{pmatrix}f_1(t) & \theta_1 & 0 & 0\\ f_2(t) & 0 & \theta_2 & 0\\ f_3(t) & 0 & 0 & \theta_3\end{pmatrix}, \tag{B2}$$

are the drift vector and the noise matrix, respectively.

It is important to highlight that each of the variables $\{z_k\}_{k=1}^3$ follows a standard Brownian motion with drift parameter $\mu_k$ and scale parameter $\theta_k$, independently of one another when there is no coupling through $\{f_k(t)\}_{k=1}^3$. Thus, the system of stochastic differential equations can be interpreted as the coupling of three independent Brownian motions with a global environment $W(t)$. Physically, this corresponds to three Langevin degrees of freedom coupled to local

baths and driven by a shared fluctuating field. Furthermore, a nonlinear coupling $m(\boldsymbol{z})$ is introduced in $z_1(t)$, representing pairwise and higher-order deterministic interactions [4].

Because the model defined by Eq. (B1) includes both nonlinear coupling and multiplicative noise; it does not admit a general analytical solution in the framework of stochastic calculus. This precludes a closed-form characterization of the trajectories of the stochastic variables. From the standpoint of statistical mechanics, one typically shifts focus from individual realizations (microscopic mechanism) to ensemble-level properties (macroscopic behavior). Thus, physical observables are computed as expectation values with respect to the underlying probability density function (PDF) governing the system dynamics.

Thence, the evolution of the probability density function associated with Eq. (B1),denoted by $\Psi(\boldsymbol{z}, t)$, is governed by the Fokker–Planck equation [5]

$$\frac{\partial \Psi}{\partial t} = -\sum_{k=1}^{3} \frac{\partial}{\partial z_k} \left[M_k(\boldsymbol{z})\, \Psi(\boldsymbol{z}, t)\right] + \frac{1}{2} \sum_{k=1}^{3} \sum_{l=1}^{3} \frac{\partial^2}{\partial z_k \partial z_l} \left[D_{kl}(t) \Psi(\boldsymbol{z}, t)\right] \tag{B3}$$

where the diffusion matrix is given by $\boldsymbol{D}(t) = \boldsymbol{F}(t)\boldsymbol{F}^T(t)$.

In the particular case where $m(\boldsymbol{z}) = 0$, and the initial condition is $\boldsymbol{z}(t_0) = \boldsymbol{z}_0 = (z_{01}, z_{02}, z_{03})$, with $t_0 \geq 0$, the partial differential equation reduces to

$$\frac{\partial \Psi}{\partial t} = -\sum_{k=1}^{3} \mu_k \frac{\partial \Psi}{\partial z_k} + \frac{1}{2} \sum_{k=1}^{3} \sum_{l=1}^{3} D_{kl}(t) \frac{\partial^2 \Psi}{\partial z_k \partial z_l} = -\boldsymbol{\mu} \cdot \boldsymbol{\nabla}_{\boldsymbol{z}} \Psi + \frac{1}{2} \boldsymbol{\nabla}_{\boldsymbol{z}}^T \boldsymbol{D}(t) \boldsymbol{\nabla}_{\boldsymbol{z}} \Psi. \tag{B4}$$

The solution to this equation in the Fourier space is

$$\Psi\left(\boldsymbol{z}, t\right) = \int_{\mathbb{R}^3} e^{i\boldsymbol{p}_{\boldsymbol{z}}^T(\boldsymbol{z}-\boldsymbol{z}_0) - i\boldsymbol{p}_{\boldsymbol{z}}^T \boldsymbol{\mu}(t-t_0) - \frac{1}{2}\int_{t_0}^{t} \boldsymbol{p}_{\boldsymbol{z}}^T \boldsymbol{D}(\tau) \boldsymbol{p}_{\boldsymbol{z}}\, d\tau} \frac{d^3 p_{\boldsymbol{z}}}{(2\pi)^3}, \tag{B5}$$

since

$$\begin{aligned}
\frac{\partial \Psi}{\partial t} &= \int_{\mathbb{R}^3} e^{i\boldsymbol{p}_{\boldsymbol{z}}^T(\boldsymbol{z}-\boldsymbol{z}_0) + \mathcal{K}(\boldsymbol{p}_{\boldsymbol{z}})} \left(\frac{d\mathcal{K}}{dt}\right) \frac{d^3 p_{\boldsymbol{z}}}{(2\pi)^3} \\
&= \int_{\mathbb{R}^3} e^{i\boldsymbol{p}_{\boldsymbol{z}}^T(\boldsymbol{z}-\boldsymbol{z}_0) + \mathcal{K}(\boldsymbol{p}_{\boldsymbol{z}})} \left(-i\boldsymbol{p}_{\boldsymbol{z}}^T \boldsymbol{\mu} + \frac{1}{2}(i\boldsymbol{p}_{\boldsymbol{z}}^T)\boldsymbol{D}(t)(i\boldsymbol{p}_{\boldsymbol{z}})\right) \frac{d^3 p_{\boldsymbol{z}}}{(2\pi)^3} \\
&= \int_{\mathbb{R}^3} e^{\mathcal{K}(\boldsymbol{p}_{\boldsymbol{z}})} \left(-\boldsymbol{\mu} \cdot \boldsymbol{\nabla}_{\boldsymbol{z}} + \frac{1}{2} \boldsymbol{\nabla}_{\boldsymbol{z}}^T \boldsymbol{D}(t) \boldsymbol{\nabla}_{\boldsymbol{z}}\right) e^{i\boldsymbol{p}_{\boldsymbol{z}}^T(\boldsymbol{z}-\boldsymbol{z}_0)} \frac{d^3 p_{\boldsymbol{z}}}{(2\pi)^3} \\
&= \left(-\boldsymbol{\mu} \cdot \boldsymbol{\nabla}_{\boldsymbol{z}} + \frac{1}{2} \boldsymbol{\nabla}_{\boldsymbol{z}}^T \boldsymbol{D}(t) \boldsymbol{\nabla}_{\boldsymbol{z}}\right) \int_{\mathbb{R}^3} e^{i\boldsymbol{p}_{\boldsymbol{z}}^T(\boldsymbol{z}-\boldsymbol{z}_0) + \mathcal{K}(\boldsymbol{p}_{\boldsymbol{z}})} \frac{d^3 p_{\boldsymbol{z}}}{(2\pi)^3} \\
&= -\boldsymbol{\mu} \cdot \boldsymbol{\nabla}_{\boldsymbol{z}} \Psi + \frac{1}{2} \boldsymbol{\nabla}_{\boldsymbol{z}}^T \boldsymbol{D}(t) \boldsymbol{\nabla}_{\boldsymbol{z}} \Psi,
\end{aligned} \tag{B6}$$

where $\mathcal{K}\left(\boldsymbol{p}\right) = -i\boldsymbol{p}^T \boldsymbol{\mu}(t-t_0) - \frac{1}{2}\int_{t_0}^{t} \boldsymbol{p}^T \boldsymbol{D}(\tau) \boldsymbol{p}\, d\tau$ is the cumulant-generating function.

Finally, noting that Eq. (B5) is a Gaussian integral; the solution of the Fokker-Planck equation in the case with $m(\boldsymbol{z}) = 0$ is the following normal multivariate distribution

$$\begin{aligned}
\Psi(\boldsymbol{z}, t) &= \frac{1}{\sqrt{(2\pi)^3 \det(\boldsymbol{C}(t))}} e^{-\frac{1}{2}(\boldsymbol{z}-\boldsymbol{M}_0(t))^T \boldsymbol{C}^{-1}(t)(\boldsymbol{z}-\boldsymbol{M}_0(t))} \\
&= \frac{1}{\sqrt{(2\pi)^3 \det(\boldsymbol{C}(t))}} \exp\left(-\frac{1}{2} \sum_{k=1}^{3} \sum_{l=1}^{3} C_{kl}^{-1}(t) \left[z_k - z_{0k} - \mu_k(t-t_0)\right] \left[z_l - z_{0l} - \mu_l(t-t_0)\right]\right).
\end{aligned} \tag{B7}$$

Here,

$$\left(\boldsymbol{M}_0\right)_k(t) = \mu_k(t-t_0), \tag{B8}$$

$$C_{kl}(t) = \delta_{kl}\theta_k\theta_l(t-t_0) + \int_{t_0}^{t} f_k(\tau) f_l(\tau) d\tau, \tag{B9}$$

are the mean vector and covariance matrix, respectively, and $\delta_{kl}$ is the Kronecker delta. Hereinafter, the case $m(\boldsymbol{z})=0$ is denominated as a *non-interacting*, $m_k > 0$, for all $k \in \{1,2,3\}$, as a *direct interaction*, and $m_k < 0$, for all $k \in \{1,2,3\}$, as a *mean-reversed interaction.*

Consequently, introducing the functions

$$h_{kl}(t) = \delta_{kl} + \frac{1}{\theta_k \theta_l (t-t_0)} \int_{t_0}^{t} f_k(\tau) f_l(\tau) d\tau, \tag{B10}$$

the correlation coefficients are

$$\rho_{kl}(t) = \frac{\delta_{kl}\theta_k\theta_l(t-t_0) + \int_{t_0}^{t} f_k(\tau) f_l(\tau) d\tau}{\sqrt{\theta_k^2(t-t_0) + \int_{t_0}^{t} f_k^2(\tau)d\tau}\sqrt{\theta_l^2(t-t_0) + \int_{t_0}^{t} f_l^2(\tau)d\tau}} = \frac{h_{kl}(t)}{\sqrt{h_{kk}(t)h_{ll}(t)}}. \tag{B11}$$

## Appendix C: No-go theorem for synergy under constant coupling to the shared environment

From the results of the previous section, we could state the following result that formalizes the statement made in the main text that purely static shared environments cannot generate synergistic information:

**Theorem C.1.** ***(No-go theorem for synergy under static shared environments)*** *For systems of three non-interacting variables, $\boldsymbol{z} = \{z_1, z_2, z_3\}$, with positive coupling to the local ($\theta_k > 0, \forall k$) and constant couplings to the shared environment ($f_k = \varphi_k$), the O-information satisfies $\Omega \geq 0$. The zero-O-information manifold, separating redundant and synergistic regimes, occurs if and only if at least one coupling to the shared environment is zero ($f_k = 0$).*

*Proof.* For constant coupling functions $\{f_k = \varphi_k\}_{k=1}^3$, the components of the covariance matrix given by Eq. (B9) satisfy

$$C_{kl} = [\delta_{kl}\theta_k\theta_l + \varphi_k\varphi_l]\, t, \tag{C1}$$

where, without loss of generality, and from now on, we take $t_0 = 0$.

Hence, the correlation coefficients are (for $k \neq l$)

$$\rho_{kl} = \frac{a_k a_l}{\sqrt{1+a_k^2}\sqrt{1+a_l^2}}, \tag{C2}$$

where the constant dimensionless ratios $a_k = \varphi_k/\theta_k$ are introduced.

Thus, all elements of the covariance matrix (B9) are proportional to $t$, while the correlation coefficients (B11) are constant. From Eq. (A6), we then obtain a constant O-information:

$$\Omega(z_1, z_2, z_3) = \frac{1}{2}\log_2\left(\frac{(1+a_1^2+a_2^2+a_3^2)(1+a_1^2)(1+a_2^2)(1+a_3^2)}{(1+a_1^2+a_2^2)(1+a_1^2+a_3^2)(1+a_2^2+a_3^2)}\right). \tag{C3}$$

From inequality

$$\begin{aligned}\left(1+a_1^2+a_2^2+a_3^2\right)\left(1+a_1^2\right)\left(1+a_2^2\right)\left(1+a_3^2\right) - \left(1+a_1^2+a_2^2\right)\left(1+a_1^2+a_3^2\right)\left(1+a_2^2+a_3^2\right)\\ = a_1^2a_2^2a_3^2\left(2+a_1^2+a_2^2+a_3^2\right) \geq 0,\end{aligned} \tag{C4}$$

it follows that

$$\frac{\left(1+a_1^2+a_2^2+a_3^2\right)\left(1+a_1^2\right)\left(1+a_2^2\right)\left(1+a_3^2\right)}{\left(1+a_1^2+a_2^2\right)\left(1+a_1^2+a_3^2\right)\left(1+a_2^2+a_3^2\right)} \geq 1. \tag{C5}$$

As a result, the O-information is always non-negative. Equality $\Omega = 0$ holds if and only if the quotient in Eq. (C5) equals one, which occurs when at least one coupling to the shared environment vanishes ($f_k = 0$ for some $k$).

□

This establishes that systems with constant couplings to the shared environment cannot generate synergistic behavior.

Theorem C.1 was proven for the case in which all variables $\boldsymbol{z}$ are coupled to their local environments with strictly positive strength ($\theta_k > 0$ for all $k$). However, redundant behavior is also the only possible outcome when the coupling to one of the local environments is turned off, whereas $\Omega$ becomes undefined when two or more of the couplings $\theta_k$ are zero.

Suppose, for example, that $\theta_1 = 0$ and $\theta_2, \theta_3 > 0$. From Eqs. (A5) and (C1), it follows that

$$\rho_{12} = \frac{\varphi_2}{\sqrt{\theta_2^2 + \varphi_2^2}}, \qquad \rho_{13} = \frac{\varphi_3}{\sqrt{\theta_3^2 + \varphi_3^2}}, \qquad \rho_{23} = \rho_{12}\rho_{13}. \tag{C6}$$

Introducing these correlation coefficients in Eq. (A6) yields

$$\Omega = \frac{1}{2}\log_2\left(\frac{1}{1-\rho_{23}^2}\right). \tag{C7}$$

Since, $\rho_{23}^2 \in [0, 1]$, Eq. (C7) shows that $\Omega \geq 0$.

When two or more of the couplings $\theta_k$ are zero, at least one of the correlation coefficients equals one, and Eq. (A5) then yields a divergent $\Omega$.

## Appendix D: Effects of time-varying coupling to fluctuating environments in non-interacting systems: Comparison of analytical and numerical results

The PDF of the dynamical system without deterministic interaction was compared with numerical simulations run using the Euler-Maruyama algorithm [6]. To ensure the accuracy of these simulations, similar orders of magnitude were used for all the elements of the covariance matrix (B9). It is worth noting that as the integration time step decreases to better capture stochastic behavior, the number of iterations in the Euler-Maruyama method increases, potentially causing a bottleneck in computational performance. To maximize computational efficiency, we parallelized our codes (see GitHub repository [7]). The O-information was derived from numerical simulations using the *HOI* Python toolbox.

Using the method of moments [8, 9], we compare the temporal evolution of the simulated elements of the means vector and the covariance matrix with the analytical solution (see Fig. 1). The set of parameters is selected to allow a smooth transition from redundancy to synergy. However, the code implemented in the simulations is independent of the shape of the temporal strength functions [7]. The values for the coefficients of determination $R^2$ and the corresponding mean absolute errors $MAE_1$ are included in each panel, quantifying the agreement between the analytical expressions and the simulated data. Panels (a)-(c) confirm the linear growth over time for the average vector predicted by Eq. (B8). Likewise, panels (d)-(f) show smooth, monotonic behavior over time for the diagonal elements of the covariance matrix, as expressed in Eq. (B9).

The largest relative differences between analytical and numerical results are observed for the off-diagonal elements of the covariance matrix $C_{12}(t)$ and $C_{23}(t)$. Note, however, that these discrepancies are small in absolute terms. In the early stages, the denominators of the relative error are very small, so even minor absolute deviations can produce large relative differences. At later times, the errors stabilize but remain slightly higher than the variances, as the cross terms accumulate numerical integration errors from $f_2(t)$ and $f_3(t)$. Moreover, because the model constrains $C_{23}(t) \sim \varphi_1\varphi_2\theta_1 \leq \max\{C_{12}(t), C_{13}(t)\}$, the off-diagonal elements are inherently more sensitive to error propagation, especially at long times.

Fig. 1(j) shows the global absolute error $GAE(t)$ defined by taking the Euclidean norm of the vector constructed with the theoretical percentage error for the 9 analytical moments ($\boldsymbol{M}_0^T(t)$ and $\left\{C_{i,j}^T(t)\right\}_{i\leq j\leq 3}$) and those obtained from the simulated data ($\boldsymbol{M}_0^S(t)$ and $\left\{C_{i,j}^S(t)\right\}_{i\leq j\leq 3}$). Mathematically, it is given by

$$GAE(t) = \sqrt{\sum_{j=1}^{3}\left|1 - \frac{M_j^T(t)}{M_j^S(t)}\right|^2 + \sum_{\substack{i<j\\ j=1}}^{3}\left|1 - \frac{C_{ij}^T(t)}{C_{ij}^S(t)}\right|^2}. \tag{D1}$$

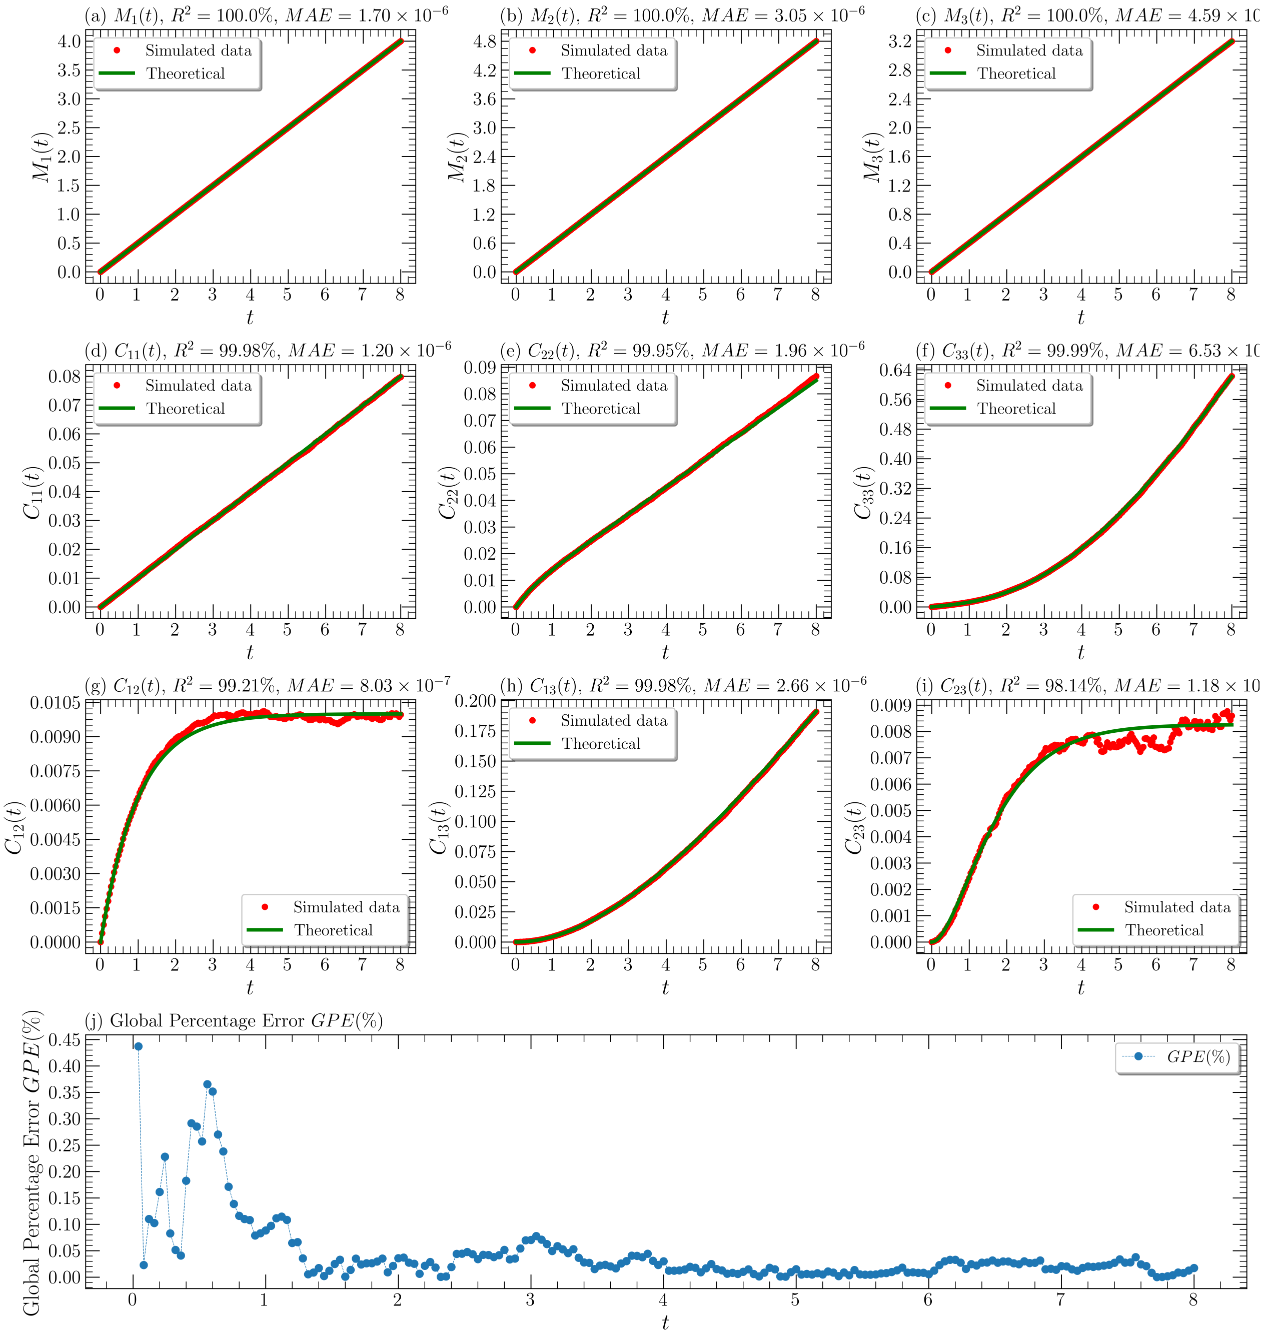


FIG. 1: Time evolution of the mean and covariance matrix of the non-interacting case. The solid green line represents the theoretical results, while the red points correspond to the simulated data. Simulations were run with parameters $\boldsymbol{\mu} = (0.5, 0.6, 0.4)$, $\boldsymbol{\theta} = (0, 0.1, 0.1)$, $\boldsymbol{\varphi} = (0.1, 0.1, 0.1)$, $\boldsymbol{\alpha} = (0, 0, 1)$, and $\boldsymbol{\beta} = (0, 1, 0.1)$, using $2 \times 10^4$ trajectories, and $4 \times 10^3$ time steps.

Relative (not absolute) mismatches dominate the $GAE(t)$, so any moment with a true value close to zero can disproportionately inflate the global absolute error. Thus, a brief hump is observed at early times because some theoretical values are close to 0, leading to an ill-conditioned percentage error. Nevertheless, for most of the time window, a low and flat $GAE(t)$ is observed (approximately 0.15%), confirming the validity of the theoretical expressions found.

Fig. 2 shows the evolution of the correlation coefficients for the same system as in Fig. 2. An excellent agreement is observed between analytical and numerical values.

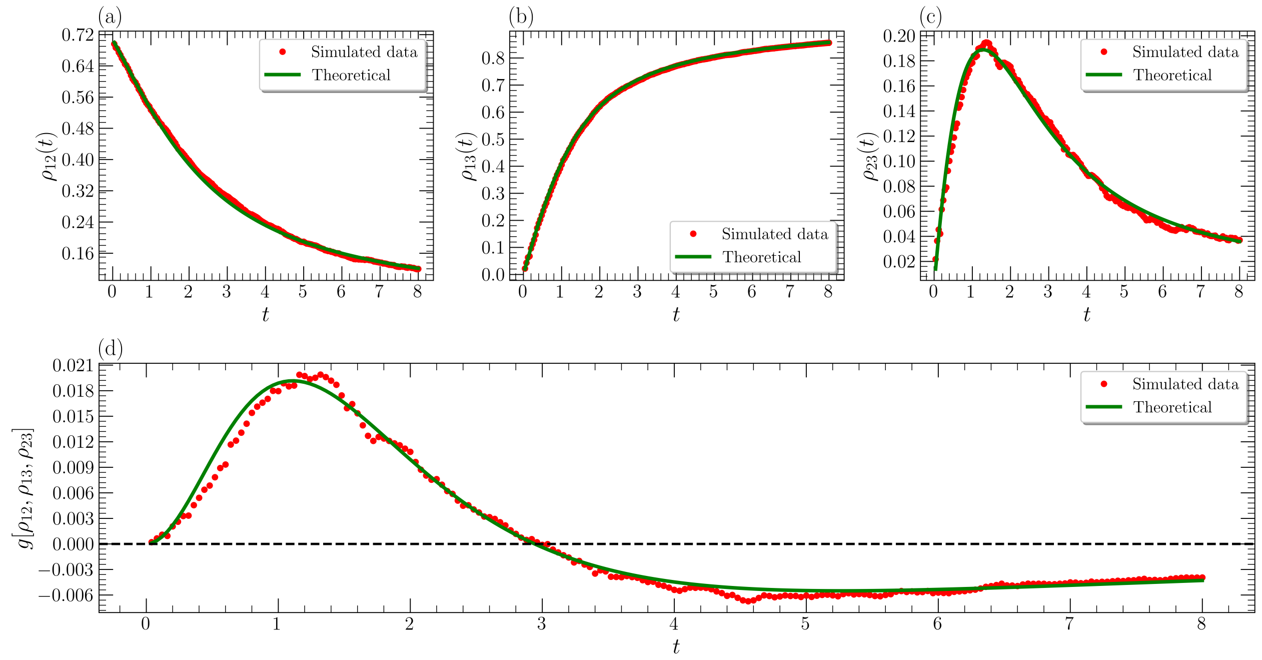


FIG. 2: Time evolution of the correlation coefficients of the non-interacting case ($m(\boldsymbol{z})=0$). The solid green line represents the theoretical results, while the red points correspond to the simulated data. Simulations were run as described in the caption of Fig. 2.


[1] F. E. Rosas, P. A. M. Mediano, M. Gastpar, and H. J. Jensen, Phys. Rev. E **100**, 10.1103/physreve.100.032305 (2019).

[2] J. Soch, K. Sarıtaş, M. Monticone, and P. Monticone, Statproofbook/statproofbook.github.io: Statproofbook 2024 (2025).

[3] N. Misra, H. Singh, and E. Demchuk, J. Multivar. Anal. **92**, 324 (2005).

[4] H. Matsuda, Phys. Rev. E **62**, 3096 (2000).

[5] D. T. Gillespie, Am. J. Phys. **64**, 1246 (1996).

[6] P. E. Kloeden and E. Platen, *Numerical Solution of Stochastic Differential Equations* (Springer Berlin Heidelberg, 1992) doi: `http://dx.doi.org/10.1007/978-3-662-12616-5`.

[7] F. Abril, GitHub repository (2025), `https://github.com/fsabrilb/O_information_toy_model`.

[8] A. Gelman, J. Comput. Graph. Stat. **4**, 36 (1995).

[9] J. Jesus and R. E. Chandler, Interface Focus **1**, 871–885 (2011).
